# Supplementary material for: Interpreting and Controlling Vision Foundation Models via Text Explanations
Source: arXiv:2310.10591 source file (2023-10-16)
Supplement: Supplementary file 1 [file supplementary.tex]

\begin{table}[t]
\centering
\small
\caption{Average Number Tokens Replaced per Layer (RS). We show the avererage number of latent tokens that are interpreted to contain the semantic of interest. For the 50 tokens in each layer of our studied transforer, we find the tokens are replaced sparsely, but the higher layers tends to be replaced more. The task for debias is slightly different in nature than the first two. In debias, we only hope to focus on one feature (hair color) and remove all other potentially spurious features, while in the first two we hope to remove/edit small details and focus on information of the entire image. Therefore, the number of tokens replaced in the last task is much larger. To prevent over-damage of image features, we only removed tokens on the final layers (which contains best quality interpretations for object-level concepts and directly contribute to CLS) and left tokens on earlier layers intact.}
\begin{tabular}{ccccccccccccc}
\toprule
Layer & 1 & 2 & 3 & 4 & 5 & 6 & 7 & 8 & 9 & 10 & 11 & 12 \\
\midrule
Typographical Attack & 0.04 & 1.04 & 0.24 & 0.27 & 0.52 & 0.46 & 0.65 & 0.76 & 0.73 & 0.53 & 0.67 & 0.48 \\
Entity Editing & 1.52 & 1.23 & 2.22 & 1.58 & 1.15 & 1.36 & 1.04 & 0.94 & 1.73 & 2.46 & 6.02 & 2.41 \\
Debias & 0 & 0 & 0 & 0 & 0 & 0 & 0 & 0 & 0 & 0 & 0 & 43.58\\
\bottomrule
\end{tabular}

\label{tab:tokens_replaced}
\end{table}

\begin{figure}[t]
\centering
% \vspace{-2em}
\includegraphics[width=.9\textwidth]{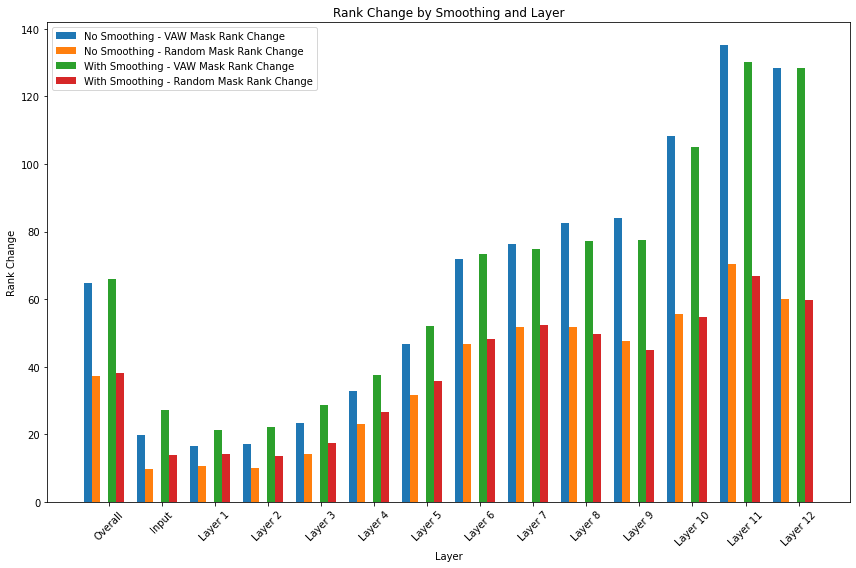}
%   \includegraphics[width=0.8\textwidth]{figures/result_lambda_matrices.pdf}
    % \vspace{-1em}
  \caption{Distribution shifts causes by our latent token intervention which disables the self-attention.}
  \label{fig:alg}
  % \vspace{-1em}
\end{figure}

\textbf{Feature Distribution Shifts}

Over the VAW and CelebA dataset, we measure the distribution shift between with attention and without attention with $L_2$ norm between the center of the distributions. We obtain the $L_2$ difference between the mean vector of tokens produced from a previous layer with attention and that from a previous layer without attention. In table/fig xx, we average the $L_2$ distance across tokens by layers. The result demonstrates that the drift is more significant at the beginning (potentially because stronger presence of positional embedding) and end (potentially because of more important token inter-relation that the model learns) of the model. In table/fig xx, we compared drift of CLS token and non-CLS token by averaging across layers. Note that we only measure the drift for layer 1 to layer 12 since interpreting layer 13 does not require disabling attention. The result shows that CLS tokens results in smaller drifts than other tokens, potentially because of lack of positonal embedding. 

\begin{table}[t]
    \caption{Average Drift}\centering
\begin{tabular}{lcc}
\hline
{} & {CLS} & {Other} \\
\hline
{CelebA} & 0.0826416015625 & 0.1031494140625 \\
{VAW} & 0.0791015625 & 0.0870361328125 \\
UC Merced Land Use (Forest) & 0.09039306640625 & 0.11492919921875\\
UC Merced Land Use (Highway) & 0.0902099609375 & 0.1019287109375\\

\hline
\end{tabular}
    \label{tab:my_label}
\end{table}

\begin{wrapfigure}{r}{0.5\textwidth}
  \includegraphics[width=1\linewidth]{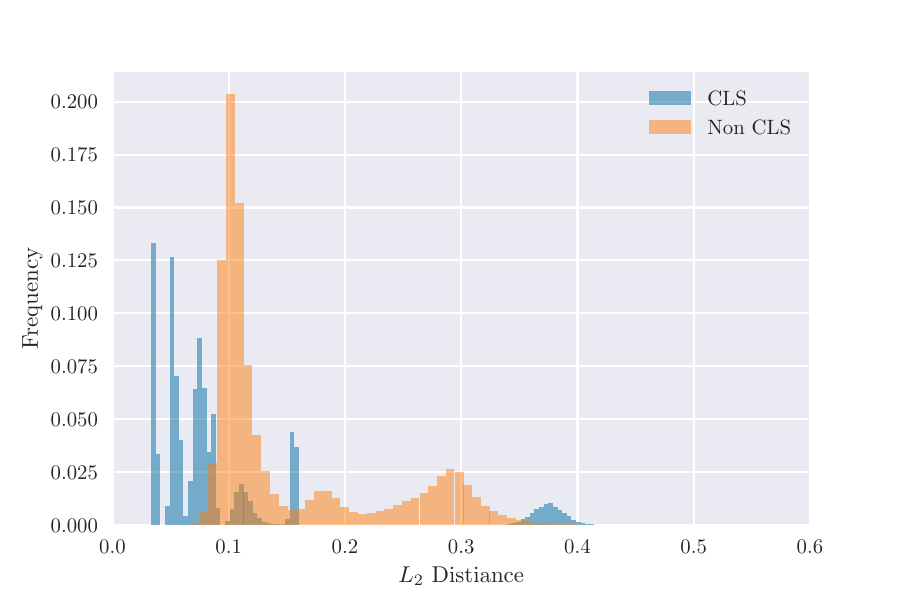}
  \caption{Distribution shifts introduced by removing cross attention. We show the histogram of the shifting for CLS token and non-CLS token separately.}  
  % when hvae time, can look at whole distribution instead of pairwise shiftsing.
  \label{fig:drifts}
\end{wrapfigure}
